# Supplementary material for: Electronic stress tensor analysis of hydrogenated palladium clusters
Source: arXiv:1110.2853 source file (2011-10-13)
Supplement: Supplementary file 1 [file supplementary_data.pdf]

# Supplementary Data

## Electronic stress tensor analysis of hydrogenated palladium clusters

**Kazuhide Ichikawa, Ayumu Wagatsuma, Paweł Szarek, Chenggang Zhou, Hansong Cheng and Akitomo Tachibana**

### Contents

Fig. S1 Structures, atom numbering and bonding patters in hydrogenated Pd-clusters.

Table S1 Lagrange point data.

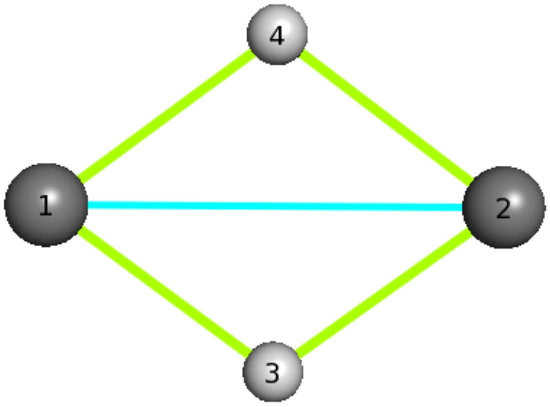


(a) $Pd_2H_2$

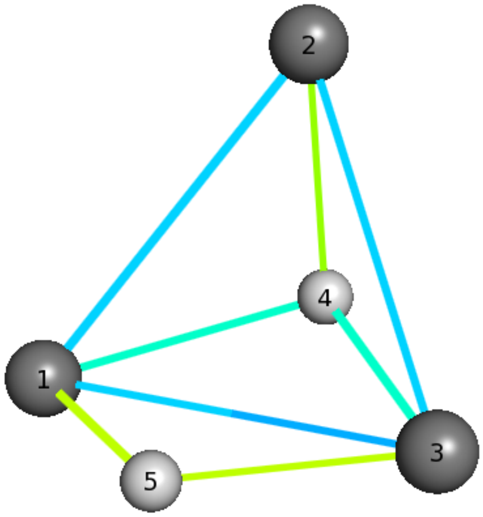


(b) $Pd_3H_2$

Fig. S1: Structures, atom numbering and bonding patters in (a) $Pd_2H_2$, (b) $Pd_3H_2$, (c) $Pd_4H_8$, (d) $Pd_5H_{10}$, (e) $Pd_6H_{14}$, (f) $Pd_7H_{16}$, (g) $Pd_8H_{16}$, (h) $Pd_9H_{22}$ .

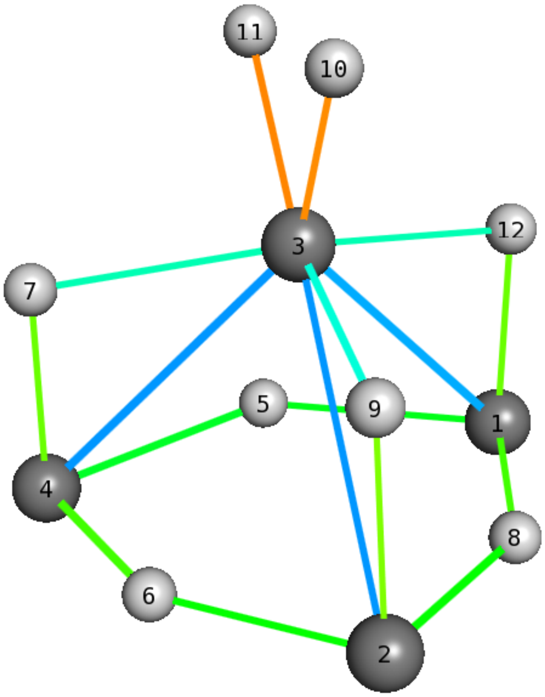


(c) $Pd_4H_8$

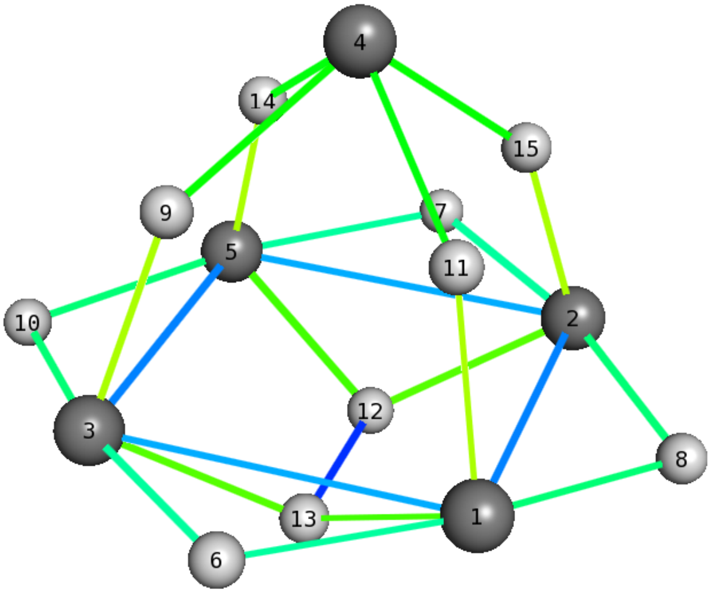


(d) $Pd_5H_{10}$

Fig. S1: (continued)

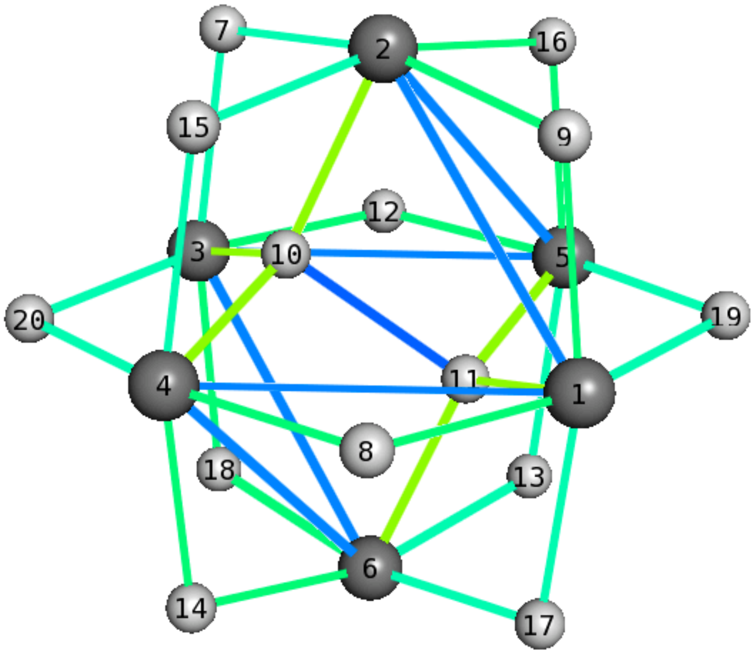


(e) $Pd_6H_{14}$

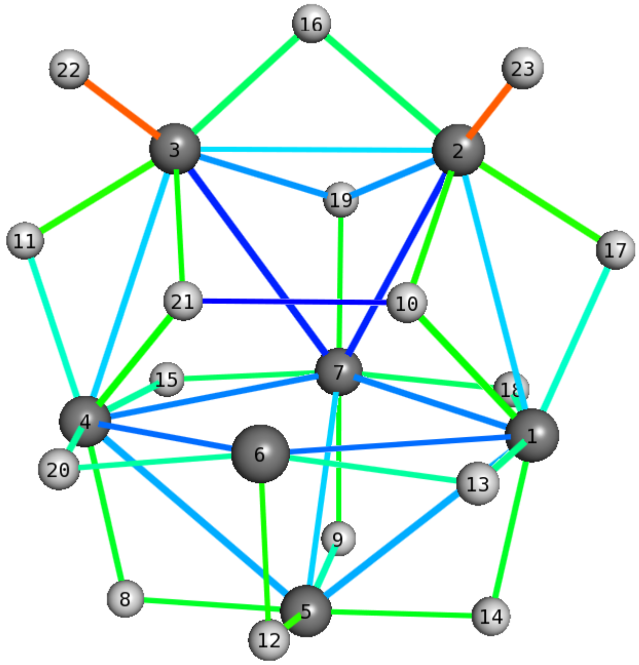


(f) $Pd_7H_{16}$

Fig. S1: (continued)

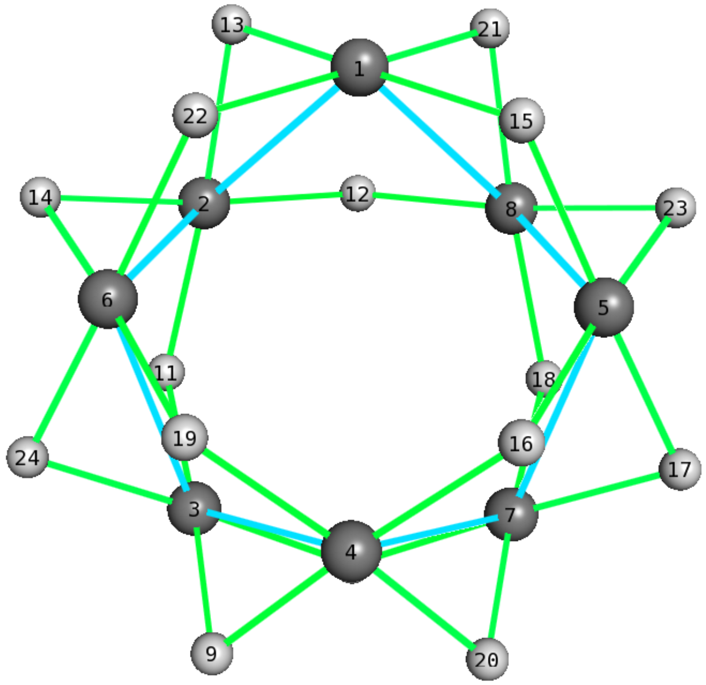


(g) $Pd_8H_{16}$

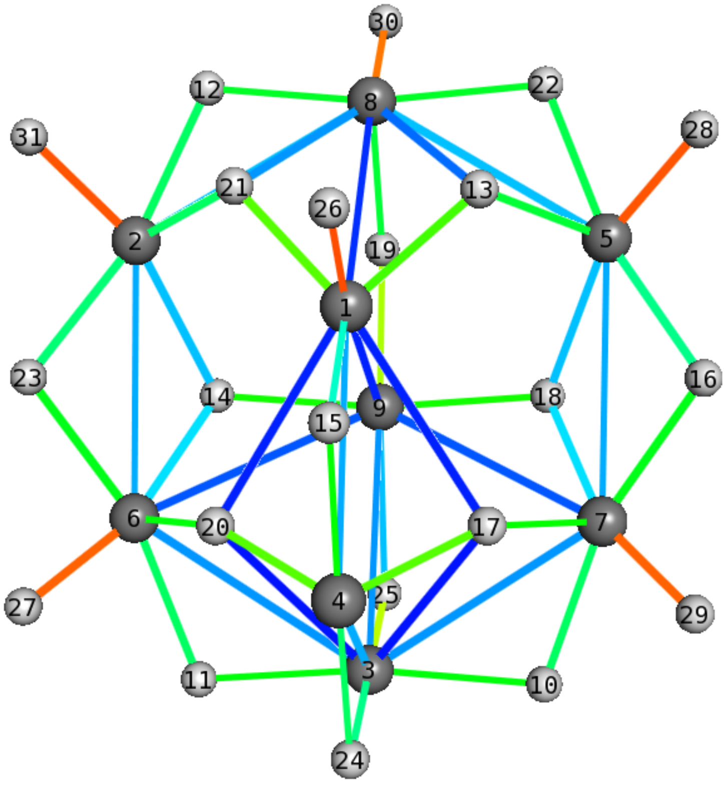


(h) $Pd_9H_{22}$

Fig. S1: (continued)

**Table S1** Lagrange point data (a)$Pd_2H_2$

| Bonding Atoms Pair | | R[Å] | b$\varepsilon$ | b$\mu$ | Wiberg index | NAO bond order | Mayer bond orders |
|---|---|---|---|---|---|---|---|
| 1 | 2 | 2.69 | 0.180 | 0.913 | 0.367 | 0.167 | 0.656 |
| 1 | 3 | 1.68 | 0.417 | 1.031 | 0.435 | 0.350 | 0.501 |
| 1 | 4 | 1.68 | 0.417 | 1.031 | 0.346 | 0.350 | 0.501 |
| 2 | 3 | 1.68 | 0.417 | 1.031 | 0.435 | 0.350 | 0.501 |
| 2 | 4 | 1.68 | 0.417 | 1.031 | 0.435 | 0.350 | 0.501 |

**Table S1** Lagrange point data (b)$Pd_3H_2$

| Bonding Atoms Pair | | R[Å] | b$\varepsilon$ | b$\mu$ | Wiberg index | NAO bond order | Mayer bond orders |
|---|---|---|---|---|---|---|---|
| 1 | 2 | 2.70 | 0.151 | 0.864 | 0.381 | 0.189 | 0.667 |
| 1 | 3 | 2.76 | 0.125 | 0.764 | 0.271 | 0.134 | 0.502 |
| 1 | 4 | 1.87 | 0.219 | 0.789 | 0.288 | 0.274 | 0.296 |
| 1 | 5 | 1.67 | 0.433 | 1.042 | 0.421 | 0.339 | 0.496 |
| 2 | 3 | 2.70 | 0.151 | 0.865 | 0.381 | 0.189 | 0.667 |
| 2 | 4 | 1.69 | 0.412 | 1.040 | 0.359 | 0.331 | 0.432 |
| 3 | 4 | 1.87 | 0.216 | 0.785 | 0.287 | 0.272 | 0.239 |
| 3 | 5 | 1.67 | 0.434 | 1.043 | 0.421 | 0.339 | 0.497 |

**Table S1** Lagrange point data (c)$Pd_4H_8$

| Bonding Atoms Pair | | R[Å] | b$\varepsilon$ | b$\mu$ | Wiberg index | NAO bond order | Mayer bond orders |
|---|---|---|---|---|---|---|---|
| 1 | 12 | 1.69 | 0.394 | 0.969 | 0.457 | 0.382 | 0.572 |
| 1 | 3 | 2.79 | 0.126 | 0.784 | 0.104 | 0.046 | 0.371 |
| 1 | 5 | 1.74 | 0.305 | 0.876 | 0.333 | 0.311 | 0.399 |
| 1 | 8 | 1.69 | 0.374 | 0.954 | 0.392 | 0.334 | 0.470 |
| 2 | 3 | 2.75 | 0.120 | 0.760 | 0.101 | 0.091 | 0.375 |
| 2 | 6 | 1.72 | 0.333 | 0.912 | 0.341 | 0.310 | 0.415 |
| 2 | 8 | 1.72 | 0.329 | 0.907 | 0.336 | 0.309 | 0.410 |
| 2 | 9 | 1.69 | 0.396 | 0.979 | 0.445 | 0.389 | 0.559 |
| 3 | 10 | 1.58 | 0.599 | 1.125 | 0.512 | 0.418 | 0.744 |
| 3 | 11 | 1.57 | 0.605 | 1.116 | 0.495 | 0.412 | 0.733 |
| 3 | 12 | 1.84 | 0.226 | 0.788 | 0.229 | 0.250 | 0.319 |
| 3 | 4 | 2.75 | 0.120 | 0.760 | 0.101 | 0.091 | 0.375 |
| 3 | 7 | 1.84 | 0.226 | 0.788 | 0.229 | 0.250 | 0.319 |
| 3 | 9 | 1.86 | 0.211 | 0.773 | 0.184 | 0.234 | 0.316 |
| 4 | 5 | 1.75 | 0.300 | 0.871 | 0.323 | 0.307 | 0.392 |
| 4 | 6 | 1.69 | 0.371 | 0.952 | 0.385 | 0.330 | 0.465 |
| 4 | 7 | 1.69 | 0.393 | 0.968 | 0.456 | 0.384 | 0.571 |

**Table S1** Lagrange point data (d)$Pd_5H_{10}$

| Bonding Atoms Pair | | R[Å] | b$\varepsilon$ | b$\mu$ | Wiberg index | NAO bond order | Mayer bond orders |
|---|---|---|---|---|---|---|---|
| 1 | 11 | 1.66 | 0.421 | 1.005 | 0.378 | 0.318 | 0.464 |
| 1 | 13 | 1.71 | 0.373 | 0.972 | 0.322 | 0.314 | 0.415 |
| 1 | 2 | 2.80 | 0.114 | 0.763 | 0.076 | 0.110 | 0.340 |
| 1 | 3 | 2.76 | 0.133 | 0.759 | 0.110 | 0.059 | 0.361 |
| 12 | 13 | 1.56 | 0.073 | 0.512 | 0.117 | 0.160 | 0.061 |
| 1 | 6 | 1.82 | 0.240 | 0.781 | 0.262 | 0.274 | 0.426 |
| 1 | 8 | 1.79 | 0.261 | 0.818 | 0.281 | 0.303 | 0.431 |
| 2 | 12 | 1.71 | 0.376 | 0.975 | 0.323 | 0.315 | 0.418 |
| 2 | 15 | 1.66 | 0.420 | 1.003 | 0.377 | 0.317 | 0.463 |
| 2 | 5 | 2.76 | 0.133 | 0.759 | 0.110 | 0.059 | 0.361 |
| 2 | 7 | 1.81 | 0.243 | 0.785 | 0.264 | 0.275 | 0.430 |
| 2 | 8 | 1.80 | 0.258 | 0.815 | 0.278 | 0.301 | 0.427 |
| 3 | 10 | 1.80 | 0.258 | 0.816 | 0.279 | 0.301 | 0.428 |
| 3 | 13 | 1.71 | 0.376 | 0.977 | 0.322 | 0.315 | 0.417 |
| 3 | 5 | 2.80 | 0.114 | 0.762 | 0.076 | 0.110 | 0.340 |
| 3 | 6 | 1.81 | 0.243 | 0.785 | 0.264 | 0.275 | 0.430 |
| 3 | 9 | 1.66 | 0.420 | 1.004 | 0.375 | 0.316 | 0.462 |
| 4 | 11 | 1.72 | 0.322 | 0.893 | 0.340 | 0.304 | 0.426 |
| 4 | 14 | 1.72 | 0.324 | 0.896 | 0.342 | 0.305 | 0.429 |
| 4 | 15 | 1.72 | 0.325 | 0.897 | 0.342 | 0.305 | 0.428 |
| 4 | 9 | 1.72 | 0.326 | 0.897 | 0.344 | 0.305 | 0.429 |
| 5 | 10 | 1.79 | 0.261 | 0.818 | 0.281 | 0.302 | 0.430 |
| 5 | 12 | 1.71 | 0.372 | 0.972 | 0.321 | 0.314 | 0.414 |
| 5 | 14 | 1.66 | 0.417 | 1.001 | 0.377 | 0.317 | 0.463 |
| 5 | 7 | 1.82 | 0.240 | 0.781 | 0.263 | 0.274 | 0.426 |

**Table S1** Lagrange point data (e)$Pd_6H_{14}$

| Bonding Atoms Pair | | R[Å] | b$\varepsilon$ | b$\mu$ | Wiberg index | NAO bond order | Mayer bond orders |
|---|---|---|---|---|---|---|---|
| 10 | 11 | 1.63 | 0.093 | 0.664 | 0.031 | 0.081 | 0.012 |
| 1 | 11 | 1.69 | 0.411 | 1.033 | 0.246 | 0.257 | 0.294 |
| 1 | 17 | 1.82 | 0.229 | 0.757 | 0.266 | 0.265 | 0.418 |
| 1 | 19 | 1.82 | 0.226 | 0.753 | 0.264 | 0.264 | 0.415 |
| 1 | 2 | 2.84 | 0.109 | 0.704 | 0.056 | 0.096 | 0.279 |
| 1 | 4 | 2.84 | 0.109 | 0.704 | 0.056 | 0.096 | 0.278 |
| 1 | 8 | 1.78 | 0.260 | 0.811 | 0.280 | 0.286 | 0.423 |
| 1 | 9 | 1.79 | 0.258 | 0.808 | 0.278 | 0.285 | 0.421 |
| 2 | 10 | 1.69 | 0.410 | 1.032 | 0.246 | 0.257 | 0.294 |
| 2 | 15 | 1.82 | 0.228 | 0.756 | 0.266 | 0.265 | 0.417 |
| 2 | 16 | 1.79 | 0.259 | 0.808 | 0.279 | 0.286 | 0.422 |
| 2 | 5 | 2.84 | 0.109 | 0.704 | 0.056 | 0.096 | 0.279 |
| 2 | 7 | 1.83 | 0.225 | 0.751 | 0.263 | 0.263 | 0.414 |
| 2 | 9 | 1.78 | 0.261 | 0.812 | 0.281 | 0.287 | 0.424 |
| 3 | 10 | 1.69 | 0.411 | 1.033 | 0.246 | 0.257 | 0.294 |
| 3 | 12 | 1.78 | 0.260 | 0.811 | 0.280 | 0.286 | 0.423 |
| 3 | 18 | 1.79 | 0.258 | 0.808 | 0.278 | 0.285 | 0.421 |
| 3 | 20 | 1.83 | 0.225 | 0.752 | 0.264 | 0.263 | 0.414 |
| 3 | 5 | 2.84 | 0.109 | 0.703 | 0.056 | 0.096 | 0.278 |
| 3 | 6 | 2.84 | 0.109 | 0.704 | 0.056 | 0.096 | 0.279 |
| 3 | 7 | 1.82 | 0.229 | 0.757 | 0.266 | 0.265 | 0.418 |
| 4 | 10 | 1.69 | 0.410 | 1.032 | 0.246 | 0.257 | 0.294 |
| 4 | 14 | 1.78 | 0.261 | 0.812 | 0.280 | 0.287 | 0.424 |
| 4 | 15 | 1.83 | 0.225 | 0.751 | 0.263 | 0.263 | 0.414 |
| 4 | 20 | 1.82 | 0.228 | 0.755 | 0.266 | 0.265 | 0.417 |
| 4 | 6 | 2.84 | 0.109 | 0.704 | 0.056 | 0.096 | 0.278 |
| 4 | 8 | 1.79 | 0.259 | 0.809 | 0.279 | 0.286 | 0.422 |
| 5 | 11 | 1.69 | 0.410 | 1.032 | 0.246 | 0.257 | 0.294 |
| 5 | 12 | 1.78 | 0.259 | 0.809 | 0.279 | 0.286 | 0.422 |
| 5 | 13 | 1.83 | 0.225 | 0.751 | 0.264 | 0.263 | 0.414 |
| 5 | 16 | 1.78 | 0.261 | 0.811 | 0.281 | 0.287 | 0.423 |
| 5 | 19 | 1.82 | 0.227 | 0.754 | 0.265 | 0.265 | 0.416 |
| 6 | 11 | 1.69 | 0.410 | 1.032 | 0.246 | 0.257 | 0.294 |
| 6 | 13 | 1.82 | 0.229 | 0.756 | 0.266 | 0.265 | 0.418 |
| 6 | 14 | 1.79 | 0.258 | 0.808 | 0.278 | 0.285 | 0.421 |
| 6 | 17 | 1.83 | 0.225 | 0.751 | 0.263 | 0.263 | 0.413 |
| 6 | 18 | 1.78 | 0.261 | 0.812 | 0.281 | 0.287 | 0.424 |

**Table S1** Lagrange point data (f)$Pd_7H_{16}$

| Bonding Atoms | Pair | R[Å] | b$\varepsilon$ | b$\mu$ | Wiberg index | NAO bond order | Mayer bond orders |
|---|---|---|---|---|---|---|---|
| 10 | 21 | 2.03 | 0.033 | 0.461 | 0.013 | 0.033 | 0.005 |
| 1 | 2 | 2.71 | 0.145 | 0.777 | 0.105 | 0.058 | 0.336 |
| 1 | 10 | 1.74 | 0.333 | 0.921 | 0.287 | 0.282 | 0.378 |
| 1 | 13 | 1.81 | 0.246 | 0.788 | 0.269 | 0.264 | 0.437 |
| 1 | 14 | 1.75 | 0.297 | 0.847 | 0.322 | 0.300 | 0.430 |
| 1 | 17 | 1.86 | 0.216 | 0.756 | 0.206 | 0.232 | 0.339 |
| 1 | 18 | 1.81 | 0.242 | 0.782 | 0.260 | 0.275 | 0.433 |
| 1 | 5 | 2.75 | 0.130 | 0.793 | 0.092 | 0.121 | 0.335 |
| 1 | 6 | 2.86 | 0.101 | 0.725 | 0.080 | 0.076 | 0.316 |
| 1 | 7 | 2.84 | 0.110 | 0.718 | 0.054 | 0.121 | 0.298 |
| 2 | 10 | 1.72 | 0.341 | 0.919 | 0.332 | 0.293 | 0.376 |
| 2 | 16 | 1.79 | 0.269 | 0.825 | 0.262 | 0.300 | 0.418 |
| 2 | 17 | 1.71 | 0.347 | 0.910 | 0.314 | 0.313 | 0.482 |
| 2 | 19 | 2.06 | 0.124 | 0.646 | 0.105 | 0.168 | 0.230 |
| 2 | 23 | 1.54 | 0.674 | 1.145 | 0.569 | 0.413 | 0.774 |
| 2 | 3 | 2.69 | 0.155 | 0.878 | 0.064 | 0.119 | 0.383 |
| 2 | 7 | 3.00 | 0.062 | 0.582 | 0.043 | 0.066 | 0.202 |
| 3 | 11 | 1.71 | 0.346 | 0.909 | 0.313 | 0.313 | 0.479 |
| 3 | 16 | 1.78 | 0.270 | 0.827 | 0.264 | 0.300 | 0.419 |
| 3 | 19 | 2.07 | 0.123 | 0.646 | 0.105 | 0.168 | 0.229 |
| 3 | 21 | 1.73 | 0.330 | 0.907 | 0.327 | 0.289 | 0.367 |
| 3 | 22 | 1.54 | 0.674 | 1.145 | 0.570 | 0.414 | 0.775 |
| 3 | 4 | 2.72 | 0.145 | 0.777 | 0.105 | 0.058 | 0.336 |
| 3 | 7 | 2.99 | 0.063 | 0.585 | 0.043 | 0.066 | 0.203 |
| 4 | 11 | 1.85 | 0.218 | 0.759 | 0.207 | 0.233 | 0.340 |
| 4 | 15 | 1.81 | 0.243 | 0.784 | 0.261 | 0.276 | 0.434 |
| 4 | 20 | 1.81 | 0.244 | 0.785 | 0.267 | 0.263 | 0.434 |
| 4 | 21 | 1.74 | 0.334 | 0.923 | 0.287 | 0.282 | 0.378 |
| 4 | 5 | 2.75 | 0.130 | 0.793 | 0.091 | 0.120 | 0.335 |
| 4 | 6 | 2.86 | 0.102 | 0.729 | 0.081 | 0.075 | 0.316 |
| 4 | 7 | 2.84 | 0.110 | 0.717 | 0.054 | 0.119 | 0.297 |
| 4 | 8 | 1.75 | 0.297 | 0.848 | 0.320 | 0.300 | 0.430 |
| 5 | 12 | 1.71 | 0.356 | 0.954 | 0.316 | 0.277 | 0.419 |
| 5 | 14 | 1.75 | 0.305 | 0.888 | 0.286 | 0.274 | 0.409 |
| 5 | 7 | 2.71 | 0.151 | 0.865 | 0.093 | 0.170 | 0.323 |
| 5 | 8 | 1.75 | 0.304 | 0.887 | 0.285 | 0.273 | 0.409 |
| 5 | 9 | 1.83 | 0.231 | 0.784 | 0.262 | 0.267 | 0.366 |
| 6 | 12 | 1.72 | 0.341 | 0.913 | 0.377 | 0.322 | 0.468 |
| 6 | 13 | 1.82 | 0.235 | 0.771 | 0.264 | 0.261 | 0.410 |
| 6 | 20 | 1.82 | 0.237 | 0.773 | 0.266 | 0.261 | 0.413 |
| 7 | 15 | 1.77 | 0.272 | 0.831 | 0.284 | 0.286 | 0.396 |
| 7 | 18 | 1.77 | 0.273 | 0.832 | 0.284 | 0.286 | 0.397 |
| 7 | 19 | 1.75 | 0.310 | 0.899 | 0.274 | 0.295 | 0.387 |
| 7 | 9 | 1.73 | 0.315 | 0.867 | 0.316 | 0.299 | 0.475 |

**Table S1** Lagrange point data (g)$Pd_8H_{16}$

| Bonding Atoms Pair | | R[Å] | b$\varepsilon$ | b$\mu$ | Wiberg index | NAO bond order | Mayer bond orders |
|---|---|---|---|---|---|---|---|
| 1 | 13 | 1.77 | 0.283 | 0.839 | 0.285 | 0.279 | 0.416 |
| 1 | 15 | 1.75 | 0.291 | 0.858 | 0.290 | 0.277 | 0.407 |
| 1 | 2 | 2.68 | 0.162 | 0.878 | 0.142 | 0.187 | 0.387 |
| 1 | 21 | 1.76 | 0.284 | 0.840 | 0.285 | 0.279 | 0.417 |
| 1 | 22 | 1.75 | 0.291 | 0.857 | 0.289 | 0.276 | 0.406 |
| 1 | 8 | 2.68 | 0.162 | 0.878 | 0.142 | 0.187 | 0.387 |
| 2 | 11 | 1.75 | 0.291 | 0.858 | 0.290 | 0.276 | 0.406 |
| 2 | 12 | 1.75 | 0.292 | 0.859 | 0.290 | 0.277 | 0.408 |
| 2 | 13 | 1.77 | 0.284 | 0.840 | 0.285 | 0.279 | 0.417 |
| 2 | 14 | 1.77 | 0.282 | 0.838 | 0.284 | 0.278 | 0.416 |
| 2 | 6 | 2.68 | 0.162 | 0.878 | 0.141 | 0.186 | 0.386 |
| 3 | 10 | 1.75 | 0.291 | 0.858 | 0.289 | 0.276 | 0.406 |
| 3 | 11 | 1.75 | 0.293 | 0.860 | 0.291 | 0.277 | 0.407 |
| 3 | 24 | 1.77 | 0.284 | 0.840 | 0.286 | 0.279 | 0.417 |
| 3 | 4 | 2.68 | 0.162 | 0.879 | 0.140 | 0.186 | 0.385 |
| 3 | 6 | 2.68 | 0.162 | 0.878 | 0.140 | 0.186 | 0.386 |
| 3 | 9 | 1.77 | 0.285 | 0.842 | 0.286 | 0.280 | 0.418 |
| 4 | 16 | 1.75 | 0.290 | 0.856 | 0.289 | 0.276 | 0.405 |
| 4 | 19 | 1.75 | 0.292 | 0.859 | 0.290 | 0.277 | 0.407 |
| 4 | 20 | 1.77 | 0.283 | 0.839 | 0.284 | 0.279 | 0.416 |
| 4 | 7 | 2.67 | 0.163 | 0.879 | 0.141 | 0.186 | 0.386 |
| 4 | 9 | 1.76 | 0.285 | 0.842 | 0.286 | 0.280 | 0.418 |
| 5 | 15 | 1.75 | 0.292 | 0.859 | 0.290 | 0.277 | 0.407 |
| 5 | 16 | 1.75 | 0.293 | 0.860 | 0.291 | 0.277 | 0.408 |
| 5 | 17 | 1.76 | 0.284 | 0.840 | 0.285 | 0.279 | 0.417 |
| 5 | 23 | 1.77 | 0.282 | 0.837 | 0.284 | 0.278 | 0.415 |
| 5 | 7 | 2.68 | 0.162 | 0.878 | 0.141 | 0.186 | 0.386 |
| 5 | 8 | 2.68 | 0.162 | 0.877 | 0.141 | 0.186 | 0.386 |
| 6 | 14 | 1.76 | 0.284 | 0.841 | 0.286 | 0.279 | 0.418 |
| 6 | 19 | 1.75 | 0.291 | 0.858 | 0.289 | 0.276 | 0.406 |
| 6 | 22 | 1.75 | 0.293 | 0.860 | 0.290 | 0.277 | 0.408 |
| 6 | 24 | 1.77 | 0.283 | 0.839 | 0.284 | 0.279 | 0.416 |
| 7 | 10 | 1.75 | 0.292 | 0.859 | 0.290 | 0.277 | 0.408 |
| 7 | 17 | 1.77 | 0.282 | 0.838 | 0.285 | 0.279 | 0.416 |
| 7 | 18 | 1.75 | 0.292 | 0.859 | 0.290 | 0.277 | 0.407 |
| 7 | 20 | 1.76 | 0.284 | 0.841 | 0.285 | 0.279 | 0.417 |
| 8 | 12 | 1.75 | 0.291 | 0.857 | 0.289 | 0.276 | 0.406 |
| 8 | 18 | 1.75 | 0.291 | 0.858 | 0.290 | 0.277 | 0.407 |
| 8 | 21 | 1.77 | 0.283 | 0.839 | 0.285 | 0.279 | 0.416 |
| 8 | 23 | 1.76 | 0.285 | 0.841 | 0.286 | 0.279 | 0.418 |

**Table S1** Lagrange point data (h)$Pd_9H_{22}$

| Bonding Atoms Pair | | R[Å] | b$\varepsilon$ | b$\mu$ | Wiberg index | NAO bond order | Mayer bond orders |
|---|---|---|---|---|---|---|---|
| 1 | 13 | 1.70 | 0.374 | 0.966 | 0.305 | 0.304 | 0.396 |
| 1 | 15 | 1.85 | 0.224 | 0.762 | 0.214 | 0.251 | 0.310 |
| 1 | 17 | 2.39 | 0.060 | 0.562 | 0.055 | 0.085 | 0.025 |
| 1 | 20 | 2.37 | 0.062 | 0.569 | 0.057 | 0.088 | 0.030 |
| 1 | 21 | 1.70 | 0.375 | 0.967 | 0.304 | 0.304 | 0.397 |
| 1 | 26 | 1.54 | 0.691 | 1.166 | 0.535 | 0.387 | 0.725 |
| 1 | 4 | 2.75 | 0.134 | 0.810 | 0.068 | 0.090 | 0.287 |
| 1 | 8 | 2.92 | 0.074 | 0.587 | 0.054 | 0.047 | 0.250 |
| 1 | 9 | 2.96 | 0.060 | 0.572 | 0.089 | 0.173 | 0.299 |
| 2 | 12 | 1.78 | 0.269 | 0.820 | 0.254 | 0.278 | 0.412 |
| 2 | 14 | 2.03 | 0.136 | 0.669 | 0.100 | 0.163 | 0.205 |
| 2 | 21 | 1.78 | 0.271 | 0.847 | 0.247 | 0.260 | 0.329 |
| 2 | 23 | 1.80 | 0.258 | 0.817 | 0.254 | 0.284 | 0.381 |
| 2 | 31 | 1.54 | 0.676 | 1.143 | 0.576 | 0.402 | 0.789 |
| 2 | 6 | 2.77 | 0.130 | 0.750 | 0.067 | 0.114 | 0.288 |
| 2 | 8 | 2.73 | 0.137 | 0.813 | 0.079 | 0.089 | 0.340 |
| 3 | 10 | 1.73 | 0.319 | 0.899 | 0.304 | 0.297 | 0.452 |
| 3 | 11 | 1.73 | 0.316 | 0.897 | 0.300 | 0.295 | 0.448 |
| 3 | 17 | 2.59 | 0.053 | 0.524 | 0.043 | 0.066 | 0.036 |
| 3 | 20 | 2.57 | 0.055 | 0.530 | 0.045 | 0.068 | 0.040 |
| 3 | 24 | 1.80 | 0.251 | 0.799 | 0.254 | 0.270 | 0.408 |
| 3 | 25 | 1.65 | 0.426 | 0.996 | 0.395 | 0.355 | 0.602 |
| 3 | 4 | 2.75 | 0.132 | 0.823 | 0.070 | 0.066 | 0.369 |
| 3 | 6 | 2.76 | 0.123 | 0.759 | 0.079 | 0.109 | 0.327 |
| 3 | 7 | 2.76 | 0.123 | 0.758 | 0.079 | 0.110 | 0.328 |
| 3 | 9 | 2.78 | 0.116 | 0.763 | 0.075 | 0.160 | 0.305 |
| 4 | 15 | 1.73 | 0.331 | 0.910 | 0.265 | 0.291 | 0.515 |
| 4 | 17 | 1.68 | 0.384 | 0.962 | 0.363 | 0.305 | 0.476 |
| 4 | 20 | 1.68 | 0.382 | 0.958 | 0.364 | 0.305 | 0.475 |
| 4 | 24 | 1.79 | 0.267 | 0.816 | 0.257 | 0.286 | 0.432 |
| 5 | 13 | 1.76 | 0.288 | 0.866 | 0.266 | 0.271 | 0.354 |
| 5 | 16 | 1.80 | 0.253 | 0.810 | 0.250 | 0.282 | 0.374 |
| 5 | 18 | 2.03 | 0.136 | 0.669 | 0.101 | 0.164 | 0.206 |
| 5 | 22 | 1.78 | 0.275 | 0.828 | 0.258 | 0.281 | 0.418 |
| 5 | 28 | 1.54 | 0.675 | 1.142 | 0.573 | 0.401 | 0.788 |
| 5 | 7 | 2.77 | 0.126 | 0.790 | 0.066 | 0.114 | 0.287 |
| 5 | 8 | 2.73 | 0.136 | 0.809 | 0.079 | 0.090 | 0.338 |
| 6 | 11 | 1.78 | 0.272 | 0.823 | 0.255 | 0.287 | 0.395 |
| 6 | 14 | 1.97 | 0.163 | 0.702 | 0.122 | 0.192 | 0.249 |
| 6 | 20 | 1.72 | 0.322 | 0.898 | 0.316 | 0.276 | 0.377 |
| 6 | 23 | 1.74 | 0.309 | 0.875 | 0.294 | 0.313 | 0.437 |
| 6 | 27 | 1.54 | 0.659 | 1.134 | 0.552 | 0.396 | 0.748 |
| 6 | 9 | 2.86 | 0.087 | 0.669 | 0.057 | 0.108 | 0.249 |
| 7 | 10 | 1.78 | 0.268 | 0.819 | 0.252 | 0.285 | 0.390 |
| 7 | 16 | 1.74 | 0.314 | 0.880 | 0.297 | 0.315 | 0.442 |
| 7 | 17 | 1.71 | 0.325 | 0.901 | 0.320 | 0.278 | 0.383 |
| 7 | 18 | 1.97 | 0.163 | 0.702 | 0.122 | 0.192 | 0.249 |
| 7 | 29 | 1.54 | 0.658 | 1.133 | 0.554 | 0.396 | 0.748 |
| 7 | 9 | 2.86 | 0.087 | 0.667 | 0.057 | 0.107 | 0.248 |
| 8 | 12 | 1.75 | 0.300 | 0.870 | 0.279 | 0.297 | 0.415 |
| 8 | 13 | 2.17 | 0.103 | 0.649 | 0.079 | 0.118 | 0.119 |
| 8 | 19 | 1.76 | 0.289 | 0.872 | 0.228 | 0.255 | 0.369 |
| 8 | 21 | 2.11 | 0.118 | 0.670 | 0.087 | 0.129 | 0.141 |
| 8 | 22 | 1.75 | 0.298 | 0.869 | 0.276 | 0.295 | 0.408 |
| 8 | 30 | 1.56 | 0.631 | 1.130 | 0.524 | 0.399 | 0.771 |
| 9 | 14 | 1.72 | 0.338 | 0.931 | 0.279 | 0.291 | 0.396 |
| 9 | 18 | 1.73 | 0.335 | 0.926 | 0.279 | 0.291 | 0.395 |
| 9 | 19 | 1.66 | 0.424 | 0.994 | 0.377 | 0.311 | 0.443 |
| 9 | 25 | 2.02 | 0.135 | 0.644 | 0.148 | 0.199 | 0.231 |
